# Supplementary material for: Multimodal Metric Learning for Tag-based Music Retrieval
Source: arXiv:2010.16030 source file (2020-10-30)
Supplement: Supplementary file 1 [file Sec0_Supplimentary.tex]

\section{Per tag AUROC on MTAT}

In Table~\ref{table:pertagauroc}, we report per tag AUROC on MTAT in a descending order. Note that our model is vulnerable to negative tags: `no voice', `no vocal', and `no vocals'.

\begin{table}[h!]
\centering
% \fontsize{7pt}{9pt}\selectfont
\small
\begin{tabular}{@{}ccccc@{}}
\toprule
metal        & choral & choir  & rock       & opera   \\
98.79        & 98.68  & 98.65  & 98.52      & 98.34   \\\midrule
flute      & harpsichord & cello        & techno    & dance    \\
97.91      & 97.85       & 96.61        & 96.51     & 96.08    \\\midrule
ambient      & piano  & harp   & country    & pop \\
95.69        & 95.69  & 95.12  & 94.05      & 94.01  \\\midrule
sitar      & man         & woman        & female    & beat     \\
93.99      & 93.70       & 93.53        & 93.41     & 93.23    \\\midrule
female vocal & male   & violin & male vocal & beats \\
92.99        & 92.91  & 92.62  & 92.34      & 92.25  \\\midrule
classical  & loud        & female voice & guitar    & quiet    \\
92.15      & 91.30       & 91.05        & 90.98     & 90.89    \\\midrule
solo         & drums  & indian & male voice & singing \\
90.36        & 89.99  & 89.99  & 89.79      & 89.77  \\\midrule
electronic & fast        & vocal        & new age   & classic  \\
89.37      & 89.15       & 88.81        & 88.73     & 88.66    \\\midrule
strings      & vocals & synth  & voice      & slow   \\
88.59        & 88.11  & 86.17  & 84.60      & 84.09   \\\midrule
soft       & weird       & no vocal     & no vocals & no voice \\
83.63      & 81.68       & 71.86        & 70.22     & 67.88    \\ \bottomrule
\end{tabular}
\vspace{0.3cm}
\caption{Per tag AUROC on MTAT}
\vspace{-0.5cm}
\label{table:pertagauroc}
\end{table}

% \begin{table*}[]
% \centering
% \fontsize{7pt}{9pt}\selectfont
% \begin{tabular}{@{}cccccccccc@{}}
% \toprule
% metal        & choral & choir  & rock       & opera   & flute      & harpsichord & cello        & techno    & dance    \\
% 98.79        & 98.68  & 98.65  & 98.52      & 98.34   & 97.91      & 97.85       & 96.61        & 96.51     & 96.08    \\\midrule
% ambient      & piano  & harp   & country    & pop     & sitar      & man         & woman        & female    & beat     \\
% 95.69        & 95.69  & 95.12  & 94.05      & 94.01   & 93.99      & 93.70       & 93.53        & 93.41     & 93.23    \\\midrule
% female vocal & male   & violin & male vocal & beats   & classical  & loud        & female voice & guitar    & quiet    \\
% 92.99        & 92.91  & 92.62  & 92.34      & 92.25   & 92.15      & 91.30       & 91.05        & 90.98     & 90.89    \\\midrule
% solo         & drums  & indian & male voice & singing & electronic & fast        & vocal        & new age   & classic  \\
% 90.36        & 89.99  & 89.99  & 89.79      & 89.77   & 89.37      & 89.15       & 88.81        & 88.73     & 88.66    \\\midrule
% strings      & vocals & synth  & voice      & slow    & soft       & weird       & no vocal     & no vocals & no voice \\
% 88.59        & 88.11  & 86.17  & 84.60      & 84.09   & 83.63      & 81.68       & 71.86        & 70.22     & 67.88    \\ \bottomrule
% \end{tabular}
% \vspace{0.3cm}
% \caption{Per tag AUROC on MTAT}
% \vspace{-0.5cm}
% \label{table:pertagauroc}
% \end{table*}

\section{More Results on Attention Heat Maps}

We report more attention heat maps of various types including voice (Figure~\ref{fig:attention_heatmap_voice}), mood (Figure~\ref{fig:attention_heatmap_mood}),  instrument (Figure~\ref{fig:attention_heatmap_inst}), and genre (Figure~\ref{fig:attention_heatmap_gnr}).

\section{Tag-wise Contribution Heat Maps}

More tag-wise contribution heat maps are illustrated in Figure~\ref{fig:tagwise_contrib_sub}.

\newpage
\begin{figure*}[ht!]
    \centering
    \begin{subfigure}[h]{0.48\linewidth}
        \centering
        \includegraphics[width=\linewidth]{figs/male_1.png}
        \caption{Tag - Male}
    \end{subfigure}
    \begin{subfigure}[h]{0.48\linewidth}
        \centering
        \includegraphics[width=\linewidth]{figs/female_2.png}
        \caption{Tag - Female}
    \end{subfigure}
    \begin{subfigure}[h]{0.48\linewidth}
        \centering
        \includegraphics[width=\linewidth]{figs/vocal_1.png}
        \caption{Tag - Vocal}
    \end{subfigure}
    \begin{subfigure}[h]{0.48\linewidth}
        \centering
        \includegraphics[width=\linewidth]{figs/novocal_1.png}
        \caption{Tag - No Vocal}
    \end{subfigure}
    % \vspace{-0.2cm}
    \caption{Attention heat maps for voice tags.}
    \label{fig:attention_heatmap_voice}
    \vspace{-0.5cm}
\end{figure*}
\begin{figure*}[ht!]
    \centering
    \begin{subfigure}[h]{0.48\linewidth}
        \centering
        \includegraphics[width=\linewidth]{figs/quiet_2.png}
        \caption{Tag - Quiet}
    \end{subfigure}
    \begin{subfigure}[h]{0.48\linewidth}
        \centering
        \includegraphics[width=\linewidth]{figs/loud_2.png}
        \caption{Tag - Loud}
    \end{subfigure}
    \begin{subfigure}[h]{0.48\linewidth}
        \centering
        \includegraphics[width=\linewidth]{figs/slow_1.png}
        \caption{Tag - Slow}
    \end{subfigure}
    \begin{subfigure}[h]{0.48\linewidth}
        \centering
        \includegraphics[width=\linewidth]{figs/fast_1.png}
        \caption{Tag - Fast}
    \end{subfigure}
    \begin{subfigure}[h]{0.48\linewidth}
        \centering
        \includegraphics[width=\linewidth]{figs/soft_1.png}
        \caption{Tag - Soft}
    \end{subfigure}
    \begin{subfigure}[h]{0.48\linewidth}
        \centering
        \includegraphics[width=\linewidth]{figs/weird_1.png}
        \caption{Tag - Weird}
    \end{subfigure}
    \caption{Attention heat maps for mood tags.}
    \label{fig:attention_heatmap_mood}
\end{figure*}

\begin{figure*}[h!]
    \centering
    \begin{subfigure}[h]{0.48\linewidth}
        \centering
        \includegraphics[width=\linewidth]{figs/cello_1.png}
        \caption{Tag - Cello}
    \end{subfigure}
    \begin{subfigure}[h]{0.48\linewidth}
        \centering
        \includegraphics[width=\linewidth]{figs/sitar_1.png}
        \caption{Tag - Sitar}
    \end{subfigure}
    \begin{subfigure}[h]{0.48\linewidth}
        \centering
        \includegraphics[width=\linewidth]{figs/harp_1.png}
        \caption{Tag - Harp}
    \end{subfigure}
    \begin{subfigure}[h]{0.48\linewidth}
        \centering
        \includegraphics[width=\linewidth]{figs/piano_2.png}
        \caption{Tag - Piano}
    \end{subfigure}
    \begin{subfigure}[h]{0.48\linewidth}
        \centering
        \includegraphics[width=\linewidth]{figs/strings_1.png}
        \caption{Tag - Strings}
    \end{subfigure}
    \begin{subfigure}[h]{0.48\linewidth}
        \centering
        \includegraphics[width=\linewidth]{figs/flute_1.png}
        \caption{Tag - Flute}
    \end{subfigure}
    \begin{subfigure}[h]{0.48\linewidth}
        \centering
        \includegraphics[width=\linewidth]{figs/drums_2.png}
        \caption{Tag - Drums}
    \end{subfigure}
    \begin{subfigure}[h]{0.48\linewidth}
        \centering
        \includegraphics[width=\linewidth]{figs/violin_1.png}
        \caption{Tag - Violin}
    \end{subfigure}
    \begin{subfigure}[h]{0.48\linewidth}
        \centering
        \includegraphics[width=\linewidth]{figs/guitar_1.png}
        \caption{Tag - Guitar}
    \end{subfigure}
    \begin{subfigure}[h]{0.48\linewidth}
        \centering
        \includegraphics[width=\linewidth]{figs/synth_1.png}
        \caption{Tag - Synth}
    \end{subfigure}
    \caption{Attention heat maps for instrument tags.}
    \label{fig:attention_heatmap_inst}
\end{figure*}

\begin{figure*}[h!]
    \centering
    \begin{subfigure}[h]{0.48\linewidth}
        \centering
        \includegraphics[width=\linewidth]{figs/classic_1.png}
        \caption{Tag - Classic}
    \end{subfigure}
    \begin{subfigure}[h]{0.48\linewidth}
        \centering
        \includegraphics[width=\linewidth]{figs/country_1.png}
        \caption{Tag - Country}
    \end{subfigure}
    \begin{subfigure}[h]{0.48\linewidth}
        \centering
        \includegraphics[width=\linewidth]{figs/opera_1.png}
        \caption{Tag - Opera}
    \end{subfigure}
    \begin{subfigure}[h]{0.48\linewidth}
        \centering
        \includegraphics[width=\linewidth]{figs/newage_1.png}
        \caption{Tag - New Age}
    \end{subfigure}
    \begin{subfigure}[h]{0.48\linewidth}
        \centering
        \includegraphics[width=\linewidth]{figs/rock_1.png}
        \caption{Tag - Rock}
    \end{subfigure}
    \begin{subfigure}[h]{0.48\linewidth}
        \centering
        \includegraphics[width=\linewidth]{figs/metal_1.png}
        \caption{Tag - Metal}
    \end{subfigure}
    \begin{subfigure}[h]{0.48\linewidth}
        \centering
        \includegraphics[width=\linewidth]{figs/pop_1.png}
        \caption{Tag - Pop}
    \end{subfigure}
    \begin{subfigure}[h]{0.48\linewidth}
        \centering
        \includegraphics[width=\linewidth]{figs/dance_1.png}
        \caption{Tag - Dance}
    \end{subfigure}
    \begin{subfigure}[h]{0.48\linewidth}
        \centering
        \includegraphics[width=\linewidth]{figs/electronic_1.png}
        \caption{Tag - Electronic}
    \end{subfigure}
    \begin{subfigure}[h]{0.48\linewidth}
        \centering
        \includegraphics[width=\linewidth]{figs/techno_1.png}
        \caption{Tag - Techno}
    \end{subfigure}
    \caption{Attention heat maps for genre tags.}
    \label{fig:attention_heatmap_gnr}
\end{figure*}

\begin{figure*}[ht!]
    \centering
    \begin{subfigure}[h]{0.48\linewidth}
        \includegraphics[width=\linewidth]{figs/female_male.png}
        \caption{Female + Male}
    \end{subfigure}
    \begin{subfigure}[h]{0.48\linewidth}
        \includegraphics[width=\linewidth]{figs/classic_metal.png}
        \caption{Classic + Metal}
    \end{subfigure}
    \begin{subfigure}[h]{0.48\linewidth}
        \includegraphics[width=\linewidth]{figs/vocal_no_vocals.png}
        \caption{Vocal + No Vocals}
    \end{subfigure}
    \begin{subfigure}[h]{0.48\linewidth}
        \includegraphics[width=\linewidth]{figs/novoice_choir.png}
        \caption{No Voice + Choir}
    \end{subfigure}
    \begin{subfigure}[h]{0.48\linewidth}
        \includegraphics[width=\linewidth]{figs/slow_fast.png}
        \caption{Slow + Fast}
    \end{subfigure}
    \begin{subfigure}[h]{0.48\linewidth}
        \includegraphics[width=\linewidth]{figs/drums_harp.png}
        \caption{Drums + Harp}
    \end{subfigure}
    \caption{Tag-wise contribution heat maps.}
    \label{fig:tagwise_contrib_sub}
\end{figure*}
